# Supplementary material for: Quantifying the consistency of scientific databases
Source: arXiv:1505.03279 source file (2015-05-13)
Supplement: Supplementary file 1 [file comparing-scientific-databases-supporting-information.pdf]

# Quantifying the Consistency of Scientific Databases

## (Supporting Information File S1)

Lovro Šubelj<sup>1</sup>, Marko Bajec<sup>1</sup>, Biljana Mileva Boshkoska<sup>2</sup>,  
Andrej Kastrin<sup>2</sup>, Zoran Levnajić<sup>1,2</sup>

<sup>1</sup> Faculty of Computer and Information Science, University of Ljubljana, Slovenia

<sup>2</sup> Faculty of Information Studies in Novo mesto, Novo mesto, Slovenia

\* Correspondence and requests for materials should be addressed to Lovro Šubelj  
(lovro.subelj@fri.uni-lj.si)

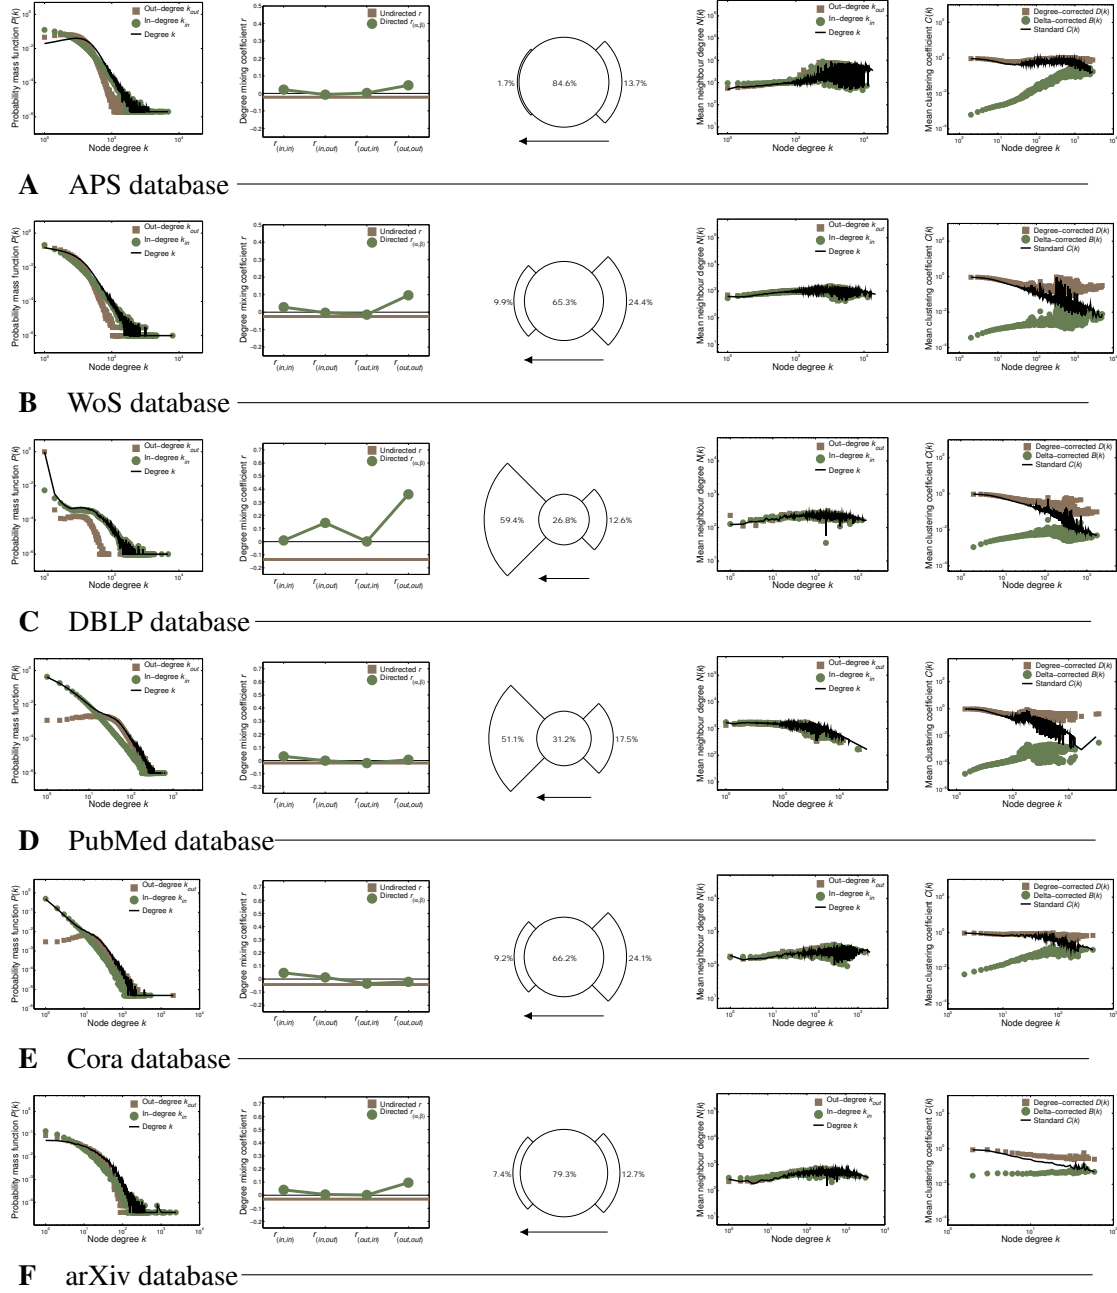

**Figure A: Degree and clustering graphical profiles.** Node degree and clustering profiles and distributions of P→P networks (first and second column), A↔A networks (third and fourth column) and A–A networks (last column). See Methods for interpretation and details on computation.

Table B1: **Continuation of network measures 1.** Degree statistics for all 18 considered networks.

| Type | Database | Degree distributions |          |               |                | Degree mixing |               |                |                |                 |
|------|----------|----------------------|----------|---------------|----------------|---------------|---------------|----------------|----------------|-----------------|
|      |          | $\langle k \rangle$  | $\gamma$ | $\gamma_{in}$ | $\gamma_{out}$ | $r$           | $r_{(in,in)}$ | $r_{(in,out)}$ | $r_{(out,in)}$ | $r_{(out,out)}$ |
| P→P  | APS      | 20.85                | 2.28     | 2.33          | 3.10           | −0.02         | 0.02          | −0.01          | 0.00           | 0.05            |
|      | WoS      | 9.97                 | 2.67     | 2.39          | 3.67           | −0.02         | 0.03          | −0.00          | −0.01          | 0.10            |
|      | DBLP     | 2.05                 | 1.80     | 1.75          | 2.82           | −0.14         | 0.01          | 0.14           | 0.00           | 0.36            |
|      | PubMed   | 6.42                 | 2.09     | 2.91          | 1.89           | −0.02         | 0.03          | 0.00           | −0.02          | 0.01            |
|      | Cora     | 6.21                 | 2.30     | 2.74          | 2.34           | −0.04         | 0.05          | 0.01           | −0.04          | −0.02           |
|      | arXiv    | 25.41                | 1.98     | 2.12          | 2.35           | −0.03         | 0.04          | 0.01           | 0.00           | 0.10            |
| A↔A  | APS      | 311.00               | 1.46     | 1.53          | 1.56           | 0.30          | 0.27          | 0.29           | 0.34           | 0.40            |
|      | WoS      | 86.31                | 1.63     | 1.71          | 1.76           | −0.01         | 0.00          | 0.00           | −0.01          | 0.01            |
|      | DBLP     | 29.46                | 1.79     | 1.97          | 1.86           | −0.04         | 0.01          | −0.01          | −0.03          | 0.00            |
|      | PubMed   | 37.31                | 1.85     | 2.08          | 1.85           | −0.02         | −0.02         | −0.02          | −0.02          | −0.02           |
|      | Cora     | 54.09                | 1.70     | 1.78          | 1.87           | 0.02          | 0.06          | 0.06           | 0.07           | 0.08            |
|      | arXiv    | 99.59                | 1.56     | 1.68          | 1.67           | −0.04         | 0.02          | 0.06           | 0.01           | 0.09            |
| A−A  | APS      | 34.00                | 1.75     | -             | -              | 0.57          | -             | -              | -              | -               |
|      | WoS      | 11.15                | 2.25     | -             | -              | 0.00          | -             | -              | -              | -               |
|      | DBLP     | 8.56                 | 2.41     | -             | -              | 0.10          | -             | -              | -              | -               |
|      | PubMed   | 20.21                | 2.12     | -             | -              | −0.01         | -             | -              | -              | -               |
|      | Cora     | 11.13                | 2.17     | -             | -              | 0.29          | -             | -              | -              | -               |
|      | arXiv    | 4.15                 | 3.45     | -             | -              | 0.13          | -             | -              | -              | -               |

Table B2: **Continuation of network measures 2.** Clustering and diameter statistics for all 18 considered networks.

| Type | Database | Clustering distributions |                      |                     | Clustering mixing |       |       | Diameter        |
|------|----------|--------------------------|----------------------|---------------------|-------------------|-------|-------|-----------------|
|      |          | $\langle c \rangle$      | $\langle b \rangle$  | $\langle d \rangle$ | $r_c$             | $r_b$ | $r_d$ | $\delta_{90}$   |
| P→P  | APS      | 0.24                     | $0.08 \cdot 10^{-2}$ | 0.28                | 0.12              | 0.43  | 0.33  | $6.91 \pm 0.05$ |
|      | WoS      | 0.15                     | $0.02 \cdot 10^{-2}$ | 0.18                | 0.22              | 0.51  | 0.44  | $8.59 \pm 0.11$ |
|      | DBLP     | 0.00                     | $0.00 \cdot 10^{-2}$ | 0.00                | 0.49              | 0.66  | 0.68  | $8.74 \pm 0.01$ |
|      | PubMed   | 0.03                     | $0.00 \cdot 10^{-2}$ | 0.04                | 0.05              | 0.41  | 0.27  | $9.02 \pm 0.12$ |
|      | Cora     | 0.11                     | $0.03 \cdot 10^{-2}$ | 0.12                | 0.07              | 0.43  | 0.33  | $7.87 \pm 0.06$ |
|      | arXiv    | 0.31                     | $0.26 \cdot 10^{-2}$ | 0.37                | 0.13              | 0.51  | 0.37  | $6.45 \pm 0.16$ |
| A↔A  | APS      | 0.39                     | $0.52 \cdot 10^{-2}$ | 0.43                | 0.38              | 0.71  | 0.74  | $4.32 \pm 0.06$ |
|      | WoS      | 0.31                     | $0.05 \cdot 10^{-2}$ | 0.34                | 0.06              | 0.12  | 0.19  | $4.79 \pm 0.03$ |
|      | DBLP     | 0.41                     | $0.41 \cdot 10^{-2}$ | 0.45                | -0.05             | 0.17  | 0.25  | $5.10 \pm 0.05$ |
|      | PubMed   | 0.28                     | $0.01 \cdot 10^{-2}$ | 0.31                | 0.11              | 0.29  | 0.28  | $4.94 \pm 0.03$ |
|      | Cora     | 0.46                     | $0.66 \cdot 10^{-2}$ | 0.51                | -0.01             | 0.34  | 0.18  | $4.79 \pm 0.04$ |
|      | arXiv    | 0.47                     | $0.70 \cdot 10^{-2}$ | 0.53                | -0.08             | 0.22  | 0.15  | $4.43 \pm 0.06$ |
| A-A  | APS      | 0.62                     | $0.76 \cdot 10^{-2}$ | 0.69                | 0.25              | 0.87  | 0.48  | $8.38 \pm 0.09$ |
|      | WoS      | 0.60                     | $0.08 \cdot 10^{-2}$ | 0.66                | 0.24              | 0.91  | 0.36  | $6.89 \pm 0.06$ |
|      | DBLP     | 0.63                     | $0.22 \cdot 10^{-2}$ | 0.70                | 0.19              | 0.84  | 0.34  | $7.81 \pm 0.03$ |
|      | PubMed   | 0.67                     | $0.01 \cdot 10^{-2}$ | 0.74                | 0.14              | 0.46  | 0.22  | $5.86 \pm 0.09$ |
|      | Cora     | 0.68                     | $1.66 \cdot 10^{-2}$ | 0.75                | 0.19              | 0.85  | 0.31  | $7.18 \pm 0.08$ |
|      | arXiv    | 0.48                     | $2.89 \cdot 10^{-2}$ | 0.57                | 0.22              | 0.64  | 0.40  | $9.31 \pm 0.07$ |
